# Supplementary material for: MVImgNet2.0: A Larger-scale Dataset of Multi-view Images
Source: arXiv:2412.01430 source file (2024-12-02)
Supplement: Supplementary file 1 [file 13_app.tex]

\section{Applications}

\paragraph{Surface Details Enhancement.} In our main paper, we demonstrate that geometric details from normal maps can be integrated into the clothing predicted by \methodName through optimization. Alternatively, we can transfer surface details from clothed humans~\cite{xiu2022icon,xiu2023econ} to garments generated by MesoCloth, forming independent clothes with geometric details~\cite{zhu2022registering,xiu2022icon}. Fig.~\ref{fig:app_sde2} provides some examples of carving geometric details from clothed humans produced by ECON~\cite{xiu2023econ} onto garments reconstructed by \methodName.

\begin{figure}[htbp]
  \centering
  \includegraphics[width=.90\linewidth]{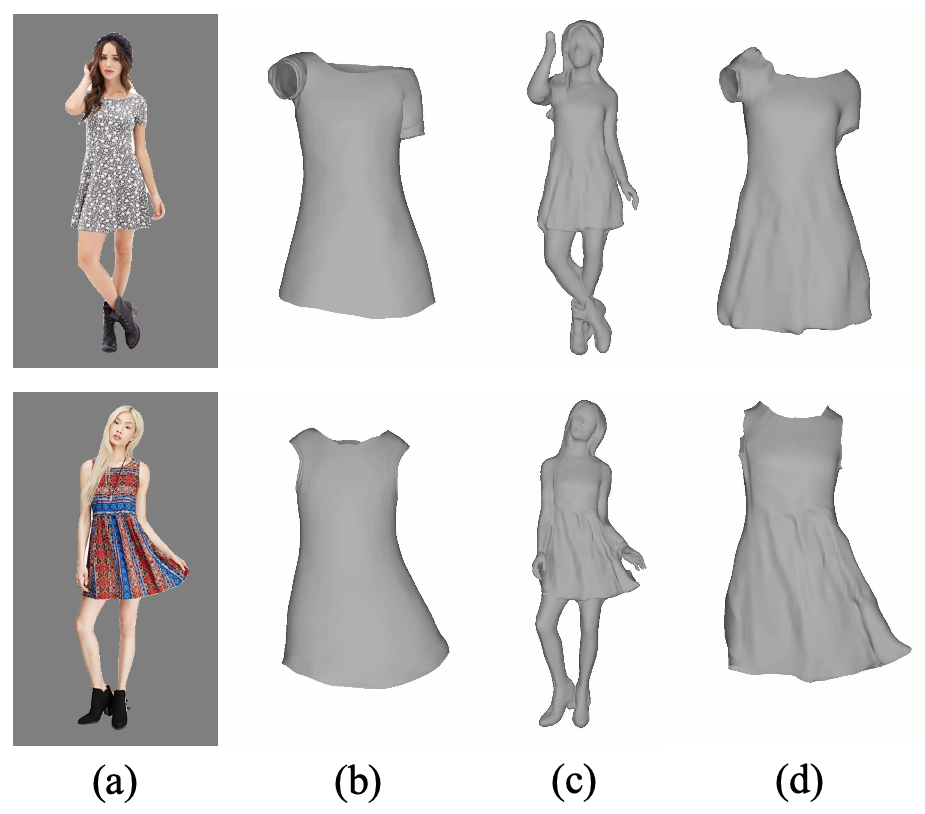}
  \caption{Examples of transferring surface details from clothed humans produced by ECON~\cite{xiu2023econ} to garments reconstructed by \methodName.}
  \label{fig:app_sde2}
\end{figure}

\paragraph{Sketch-Based Garment Editing.} We have shown how to enhance garments reconstructed by \methodName using text-to-3D techniques in the main paper. Additionally, garments recovered by \methodName  can also be edited through sketch-based modeling approaches~\cite{li2018robust,li2017bendsketch,luo2021simpmodeling,luo2023sketchmetaface}. We conduct an experiment on adopting the strategy proposed by SimpModeling~\cite{luo2021simpmodeling} to sketch-based garment editing. Specifically, given a garment reconstructed by \methodName, we render its 2D sketch, as well as the front and back view depth maps. Subsequently, we modify the 2D sketch (e.g., adding strokes to depict geometric details) and learn a pixel-aligned implicit field~\cite{saito2019pifu,chibane2020neural,qiu2023recmv} from the refined sketch and the rendered depth maps. Fig.~\ref{fig:app_sbe} illustrates some examples of sketch-based garment editing.

\begin{figure}[htbp]
  \centering
  \includegraphics[width=.99\linewidth]{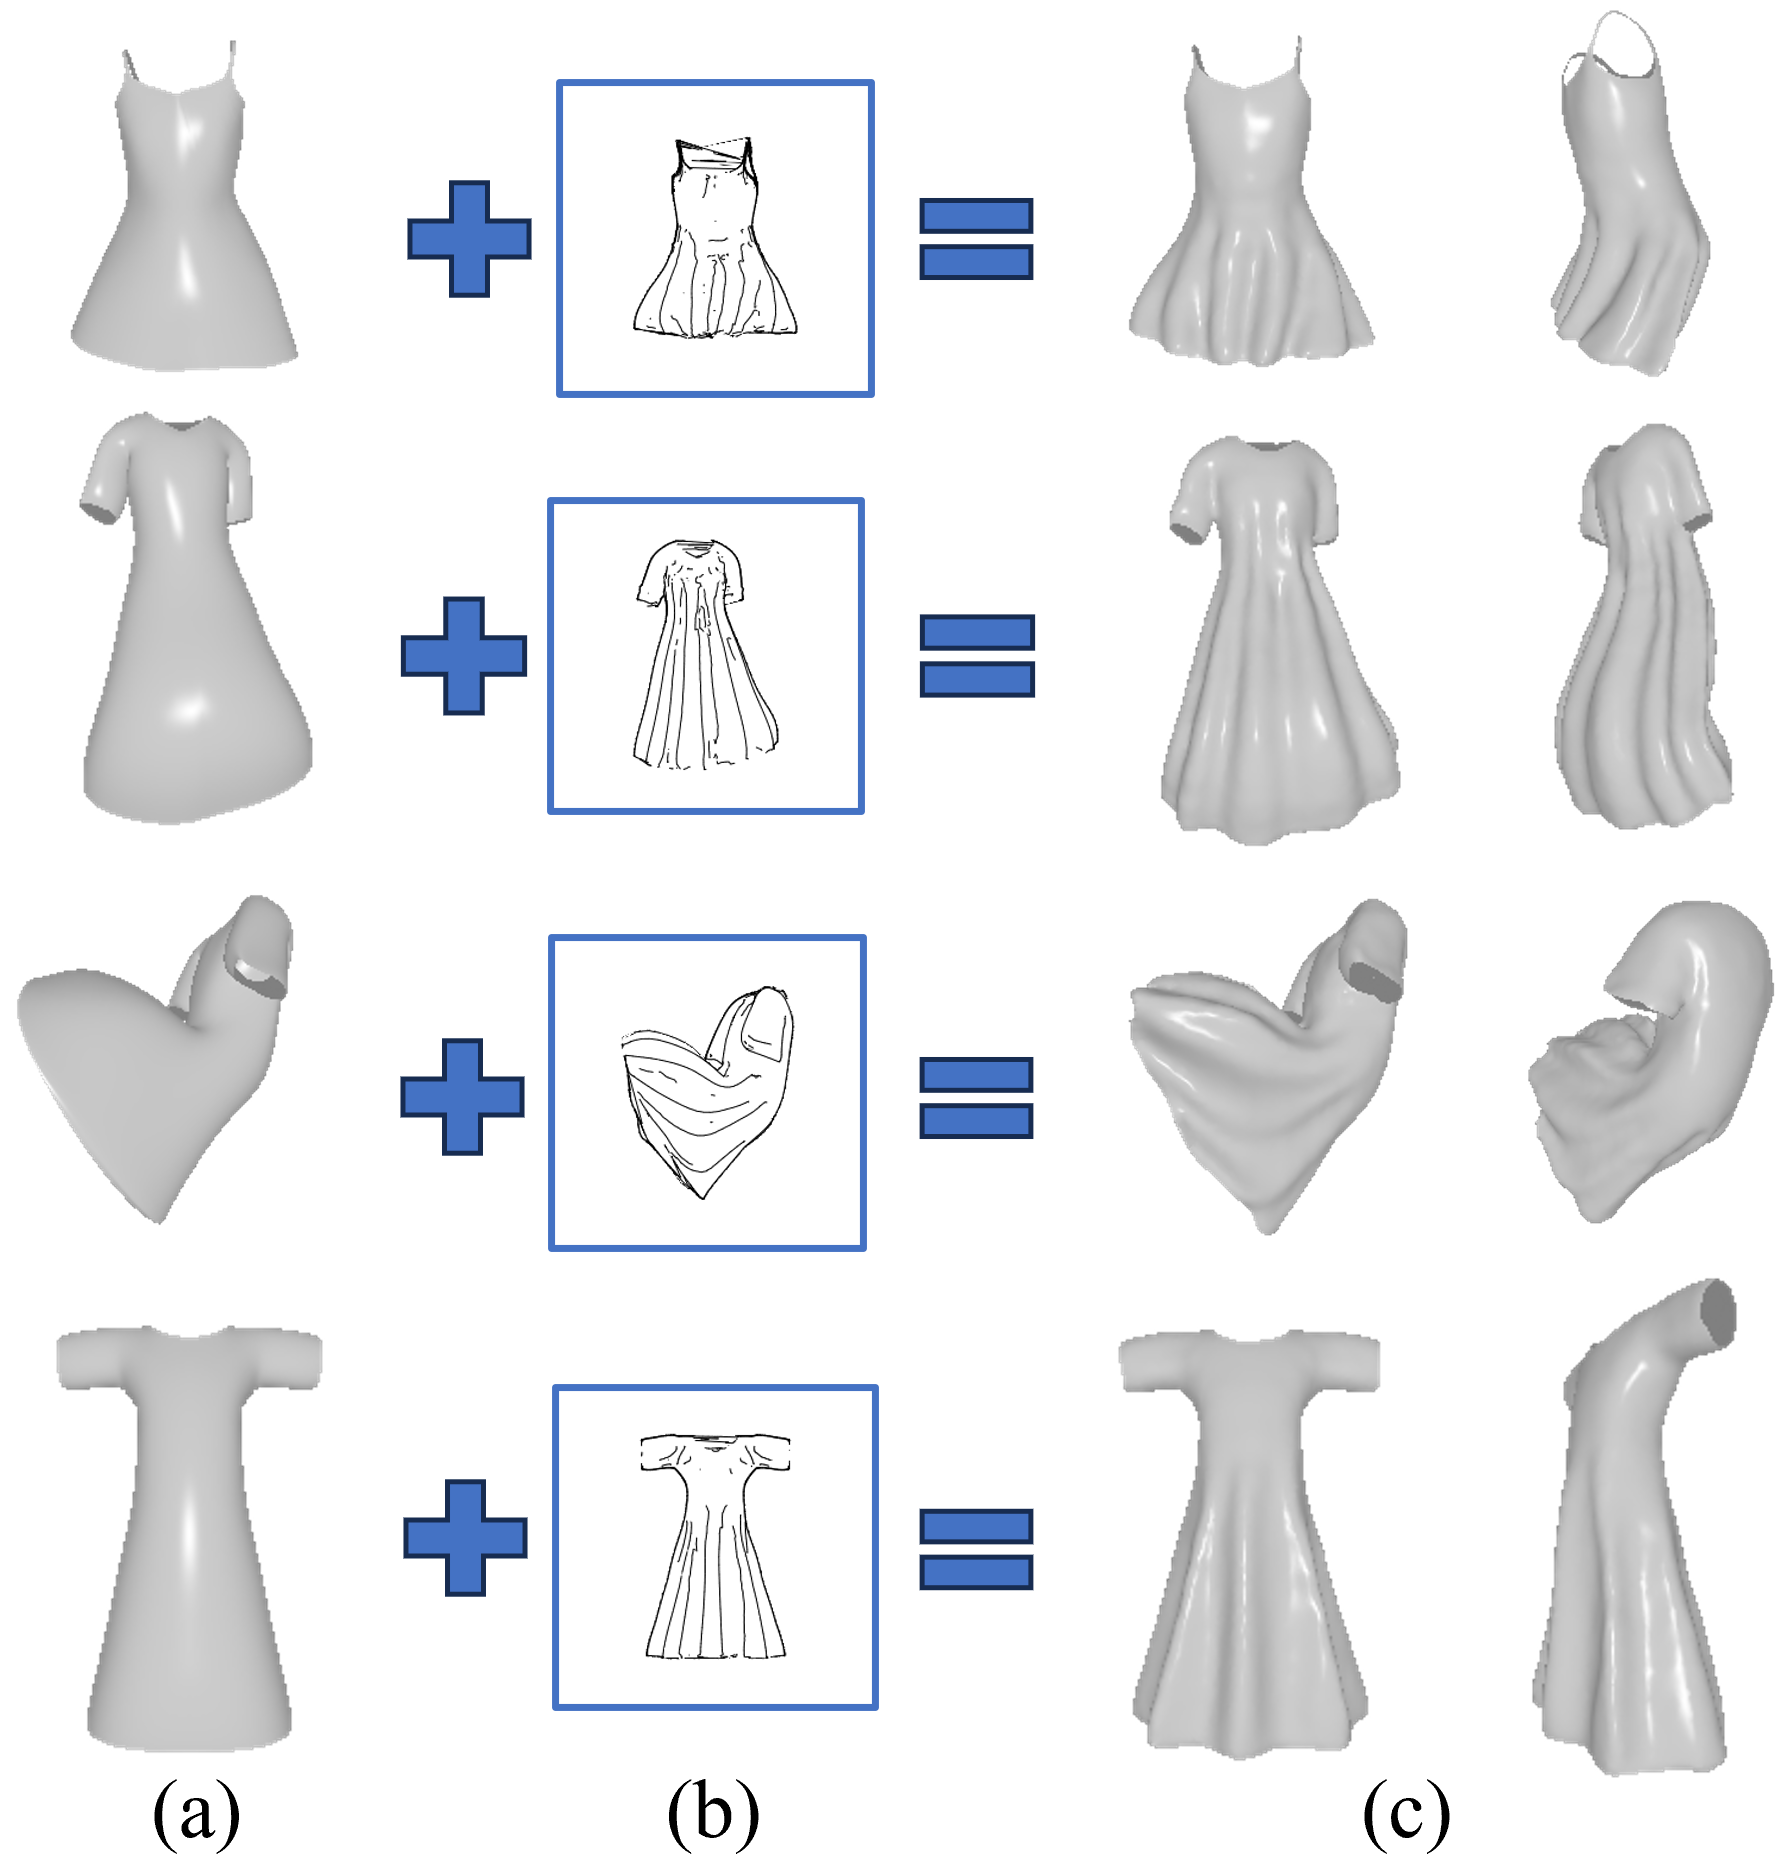}
  \caption{An illustration of sketch-based garment editing. Given a garment  (a) reconstructed by \methodName, we can further sculpt geometric details (c) onto it with a detailed sketch (b).}
  \label{fig:app_sbe}
\end{figure}
