# Supplementary material for: MVImgNet2.0: A Larger-scale Dataset of Multi-view Images
Source: arXiv:2412.01430 source file (2024-12-02)
Supplement: Supplementary file 2 [file fig_ablation2.tex]

\begin{figure*}[htbp]
  \centering
  \includegraphics[width=.93\linewidth]{images/fig_compare2.png}
  \caption{Qualitative comparison between our method and the optional strategies for modeling pose-independent meso-scale deformation. For each case, the input image (a) is followed by the results generated by (b) the displacement-based method, (c) the feature-line-based method, and (d) our method.}
  \label{fig:data_ablation2}
\end{figure*}
