# Supplementary material for: MVImgNet2.0: A Larger-scale Dataset of Multi-view Images
Source: arXiv:2412.01430 source file (2024-12-02)
Supplement: Supplementary file 3 [file fig_app_sbe.tex]

\begin{figure}[htbp]
  \centering
  \includegraphics[width=.99\linewidth]{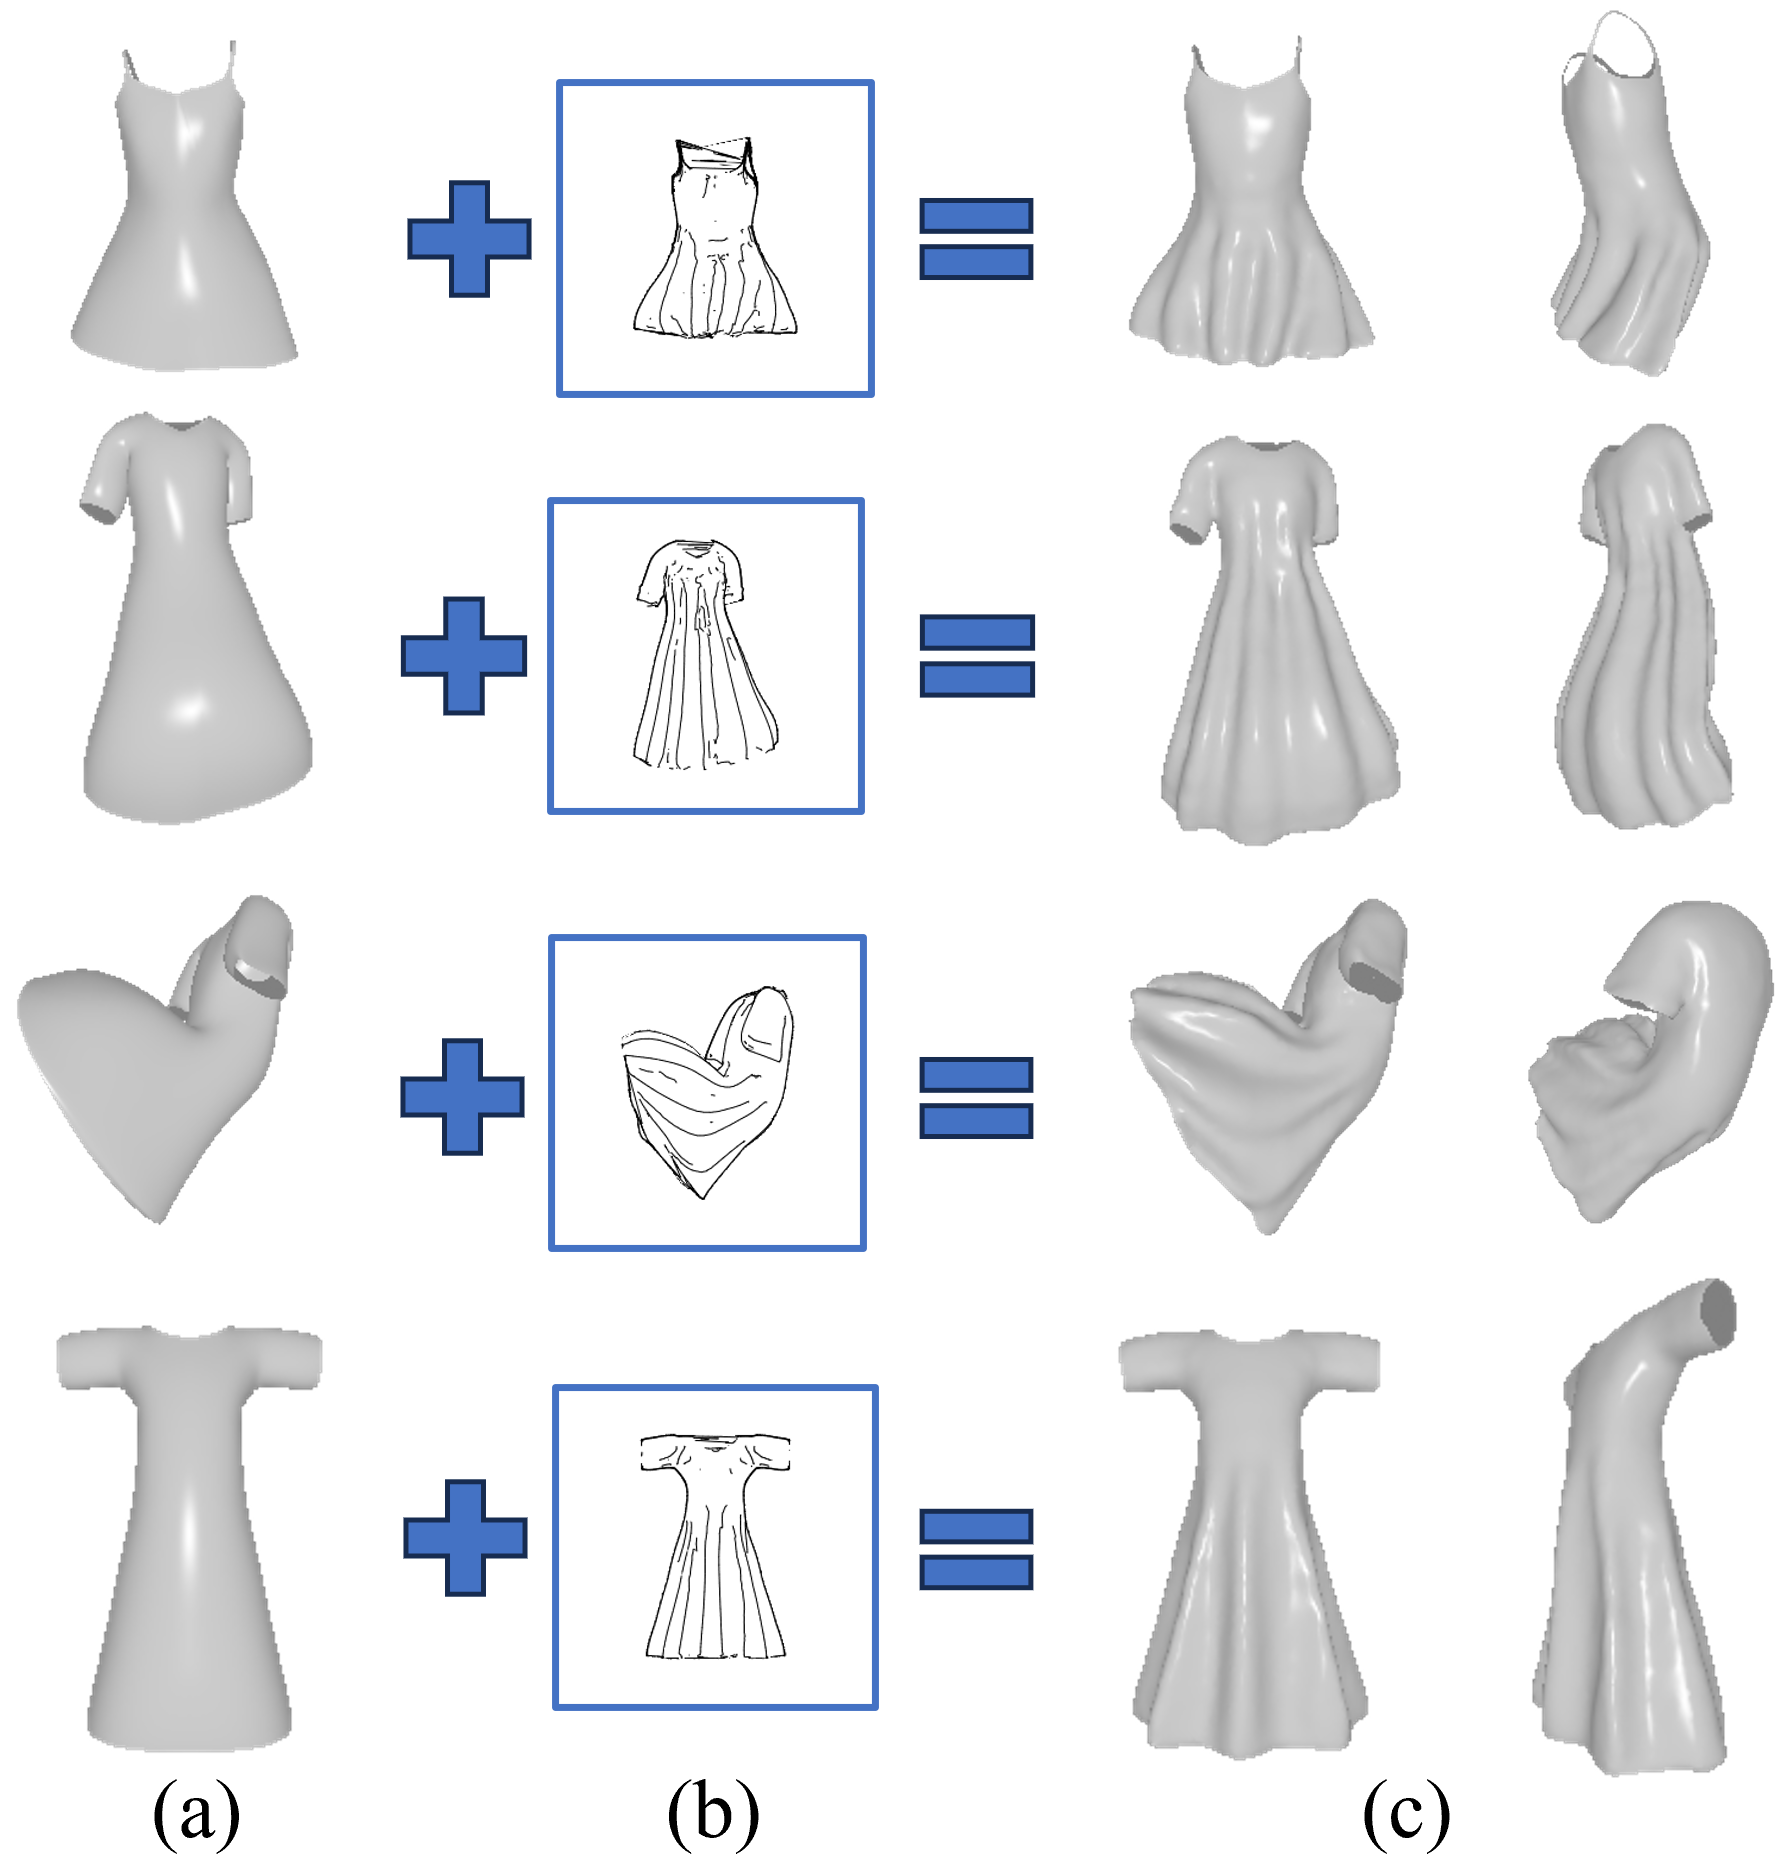}
  \caption{An illustration of sketch-based garment editing. Given a garment  (a) reconstructed by \methodName, we can further sculpt geometric details (c) onto it with a detailed sketch (b).}
  \label{fig:app_sbe}
\end{figure}
