# Supplementary material for: MVImgNet2.0: A Larger-scale Dataset of Multi-view Images
Source: arXiv:2412.01430 source file (2024-12-02)
Supplement: Supplementary file 4 [file fig_app_sde2.tex]

\begin{figure}[htbp]
  \centering
  \includegraphics[width=.90\linewidth]{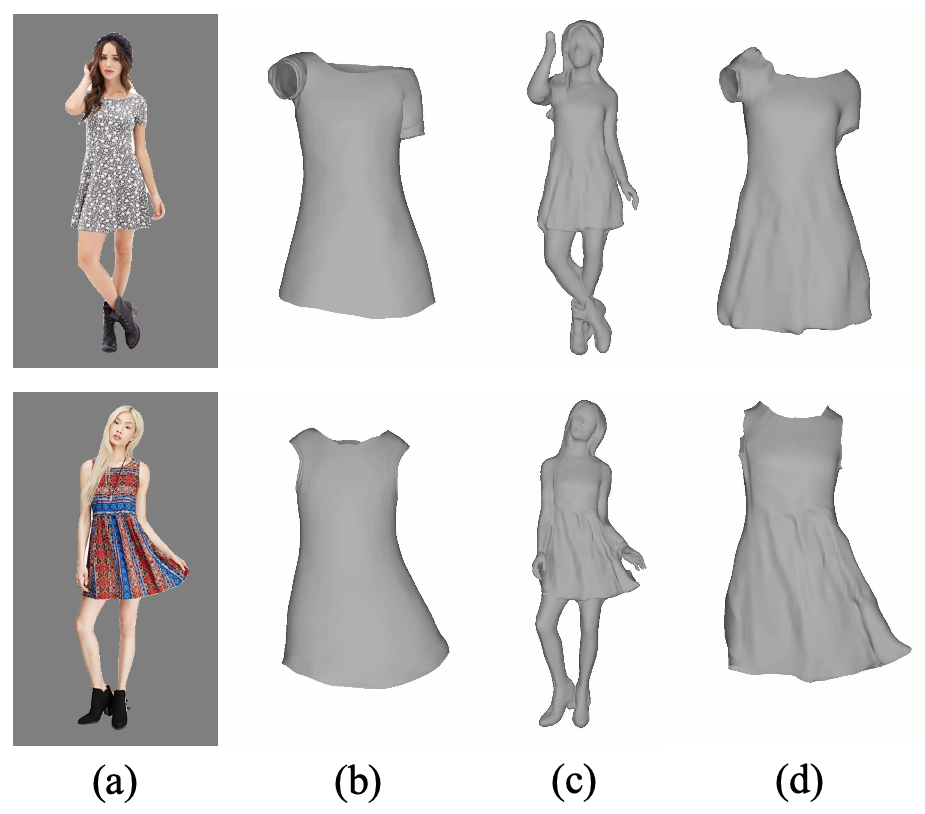}
  \caption{Examples of transferring surface details from clothed humans produced by ECON~\cite{xiu2023econ} to garments reconstructed by \methodName.}
  \label{fig:app_sde2}
\end{figure}
