# Supplementary material for: MVImgNet2.0: A Larger-scale Dataset of Multi-view Images
Source: arXiv:2412.01430 source file (2024-12-02)
Supplement: Supplementary file 5 [file fig_wr_data.tex]

\begin{figure}[htbp]
  \centering
  \includegraphics[width=.98\linewidth]{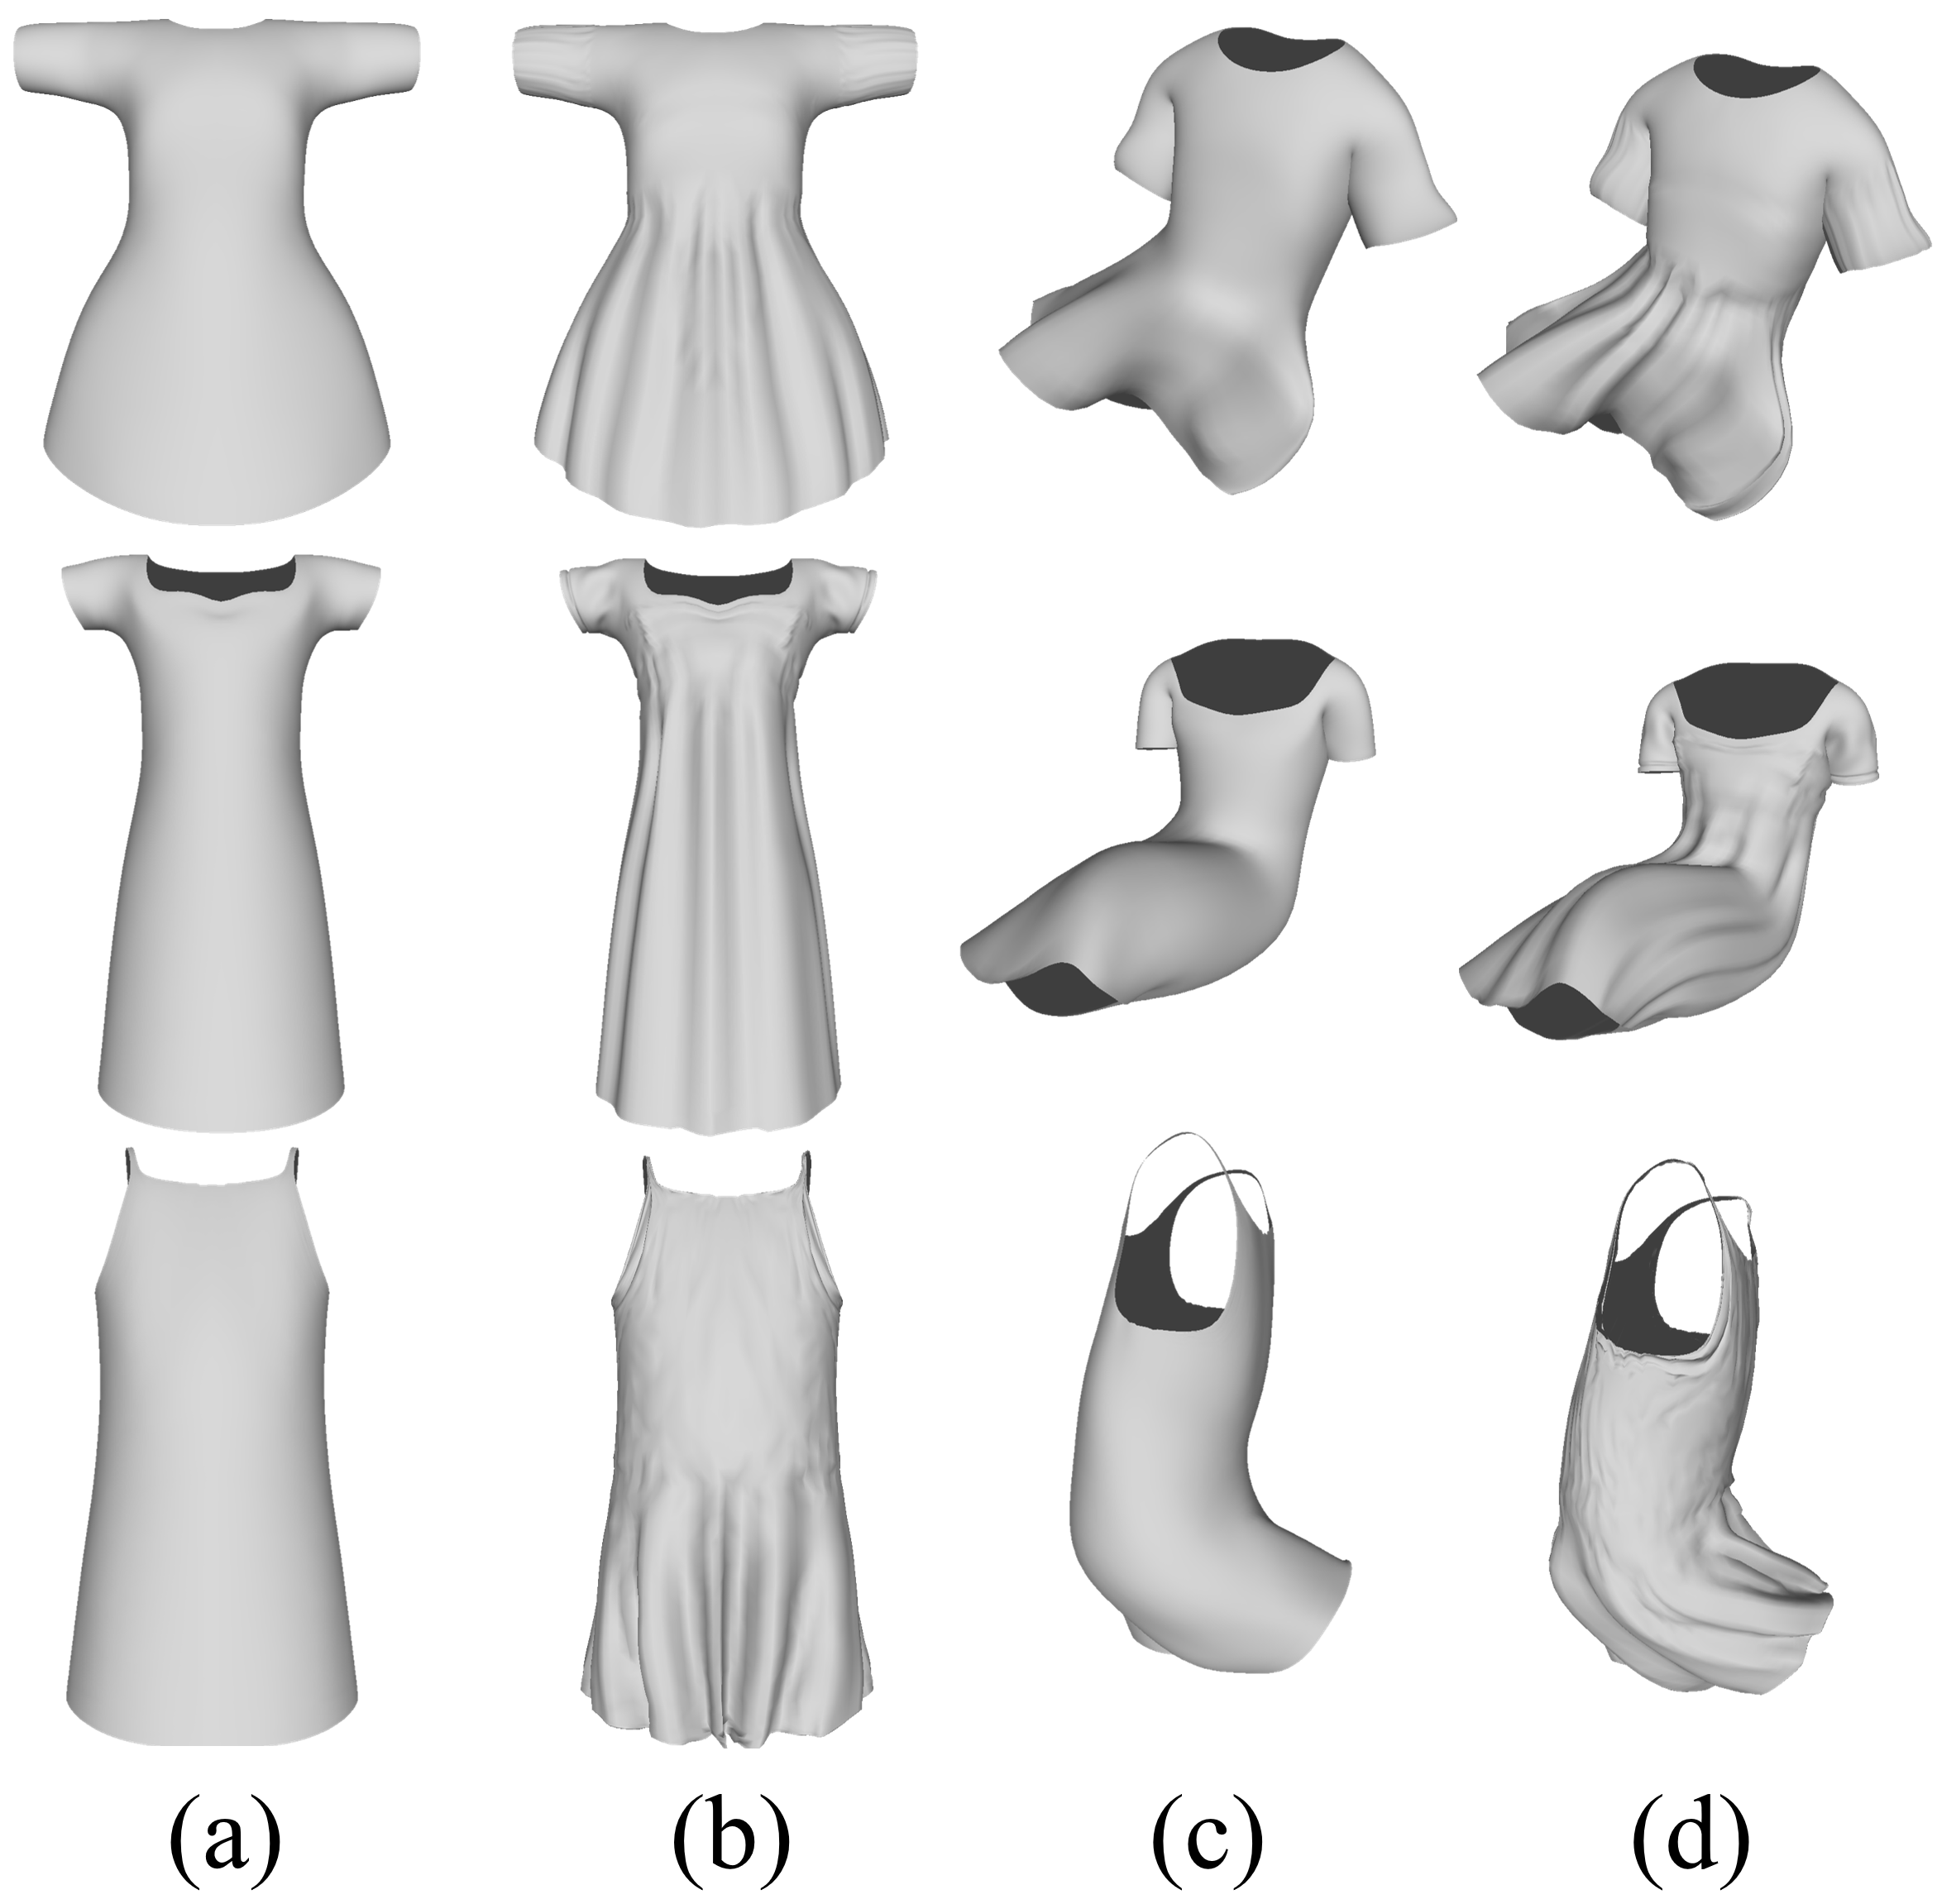}
  \caption{Given a T-posed garment (a) in \dataName, artists are required to sculpt geometric details (b) on it. Then these surface details are transferred programmatically to the corresponding garment with meso-scale deformations (c) to obtain the final garment (d).}
  \label{fig:wr_data}
\end{figure}
