# Supplementary material for: MVImgNet2.0: A Larger-scale Dataset of Multi-view Images
Source: arXiv:2412.01430 source file (2024-12-02)
Supplement: Supplementary file 6 [file fig_wr_t2i.tex]

\begin{figure}[htbp]
  \centering
  \includegraphics[width=.98\linewidth]{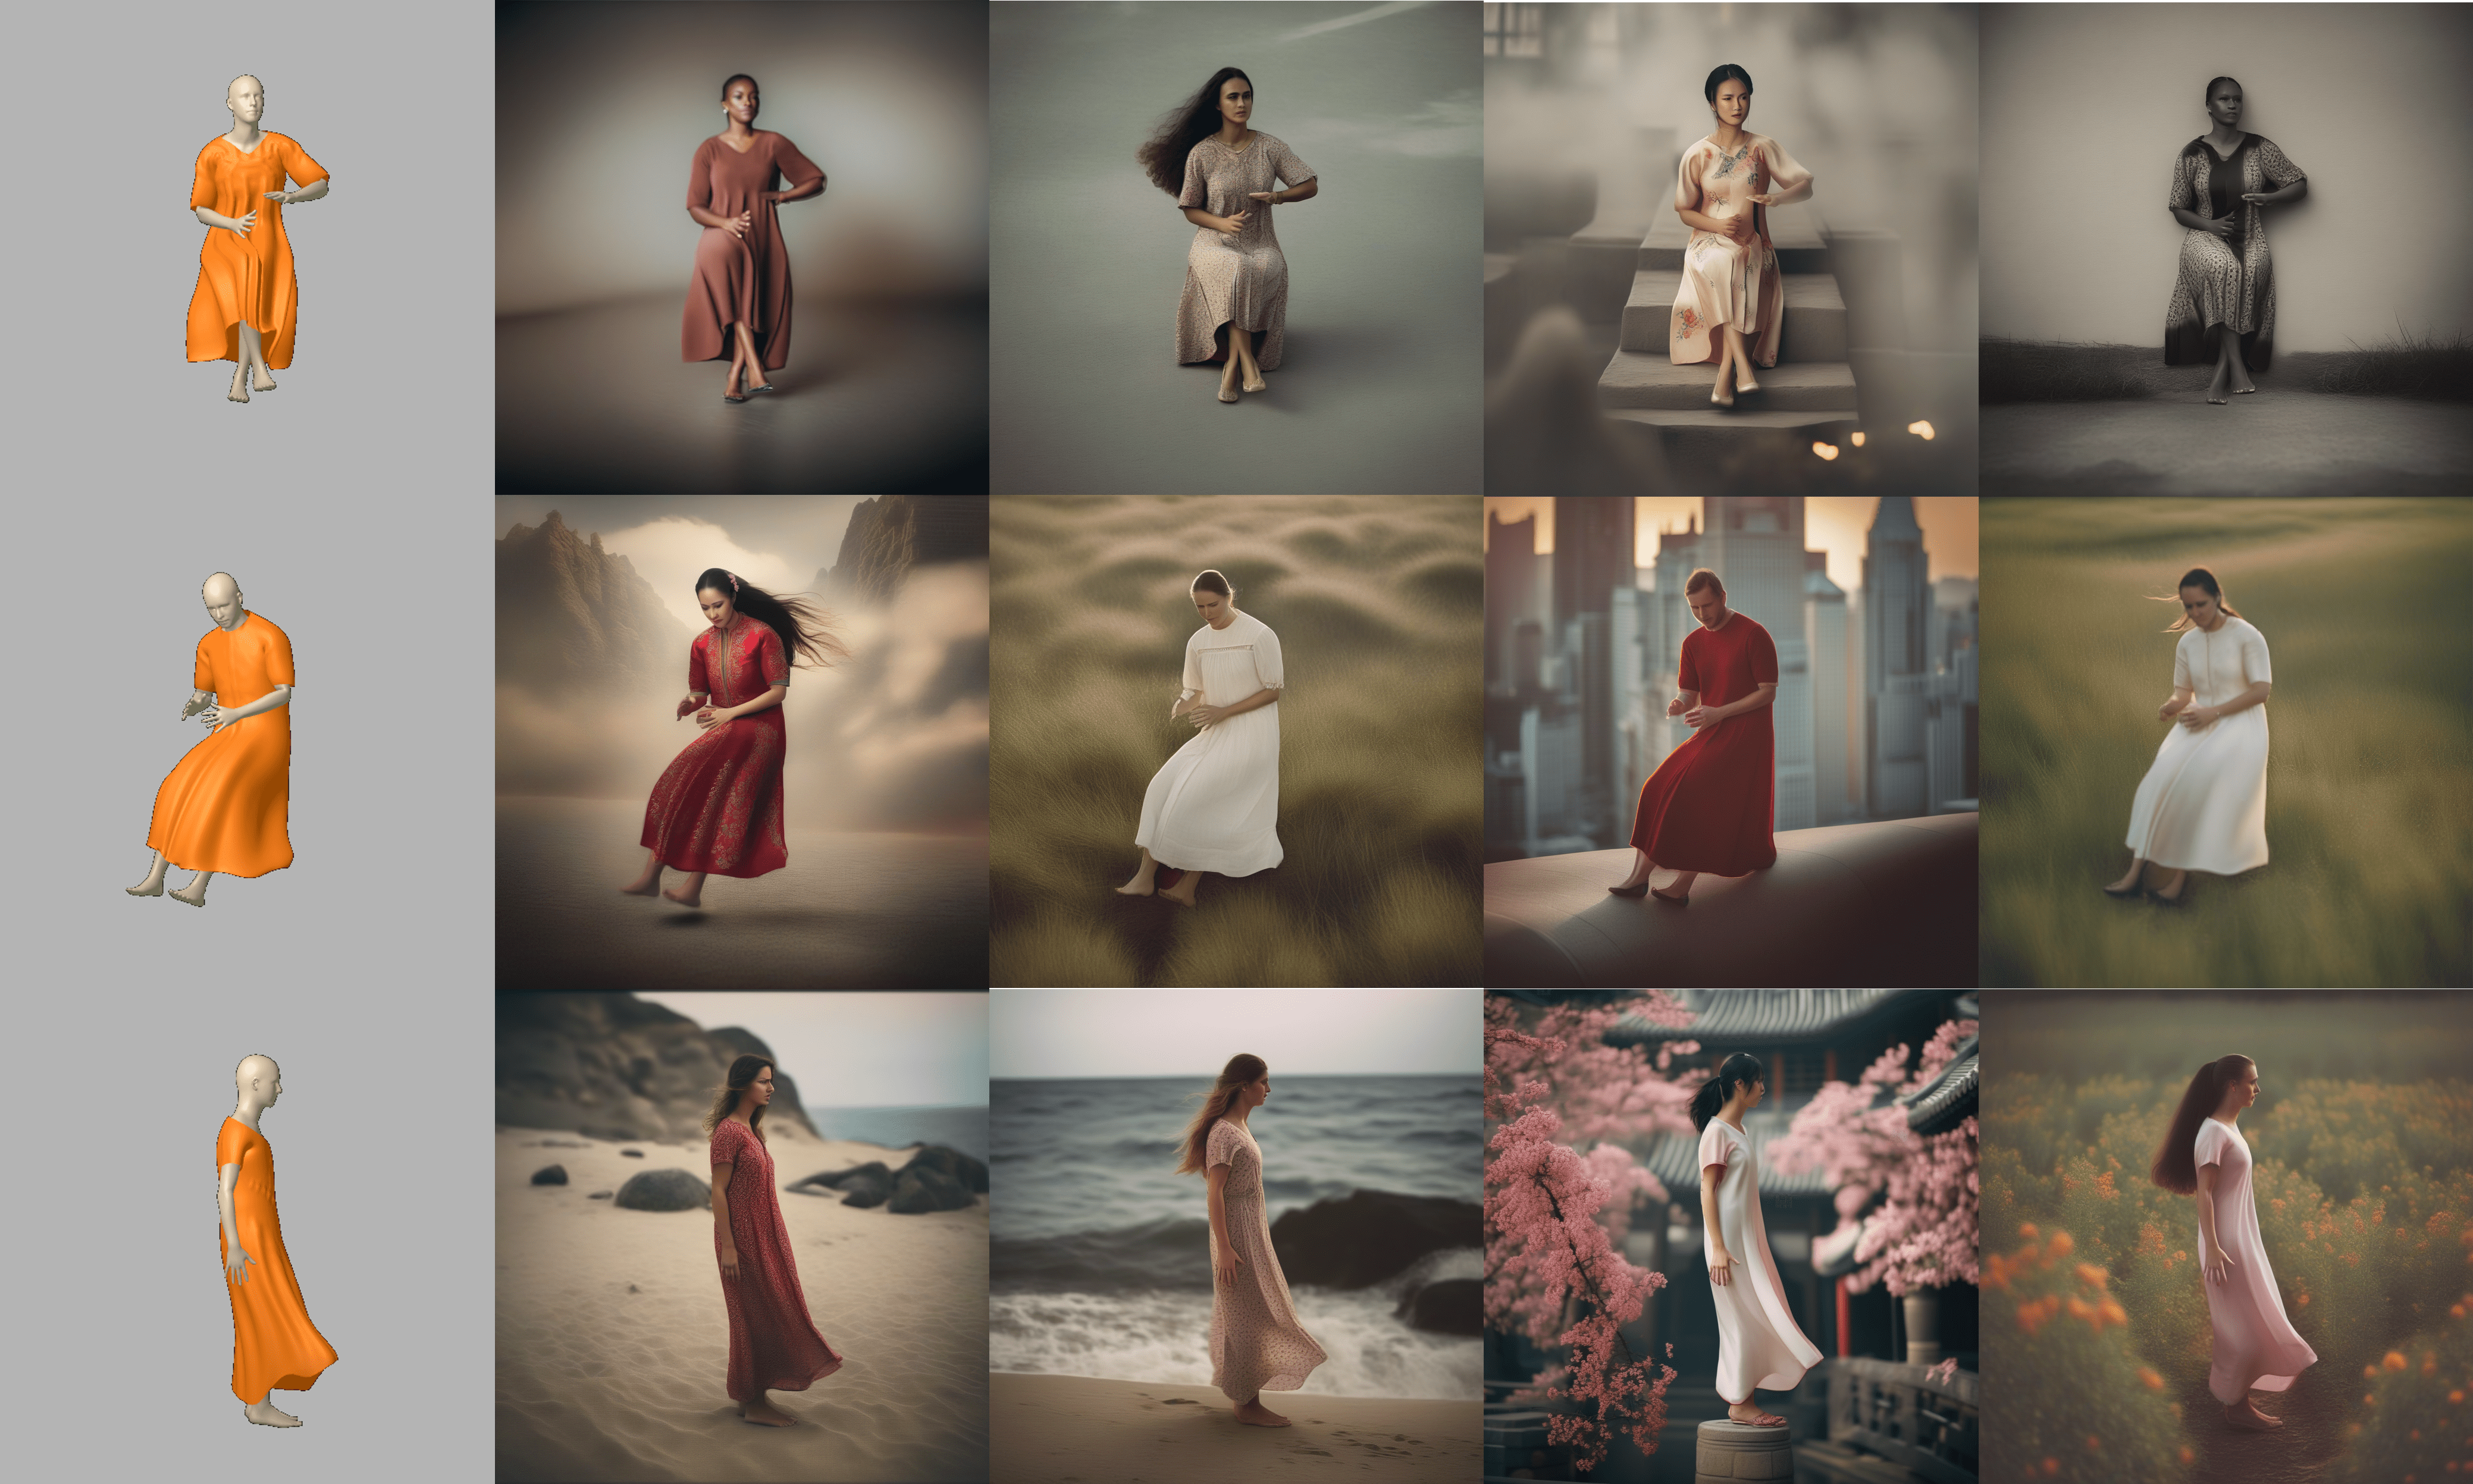}
  \caption{Sampled images generated by ControlNet~\cite{zhang2023adding} and T2I-Adapter~\cite{mou2023t2i}. For each row, the 3D garment is followed by four generated images. While these models perform well in generating images with correct global meso-scale deformations, producing images with precise fine-grained geometric details aligned with 3D garments remains challenging.}
  \label{fig:wr_t2i}
\end{figure}
