# Supplementary material for: MVImgNet2.0: A Larger-scale Dataset of Multi-view Images
Source: arXiv:2412.01430 source file (2024-12-02)
Supplement: Supplementary file 7 [file fig_wr_training_result.tex]

\begin{figure}[htbp]
  \centering
  \includegraphics[width=.98\linewidth]{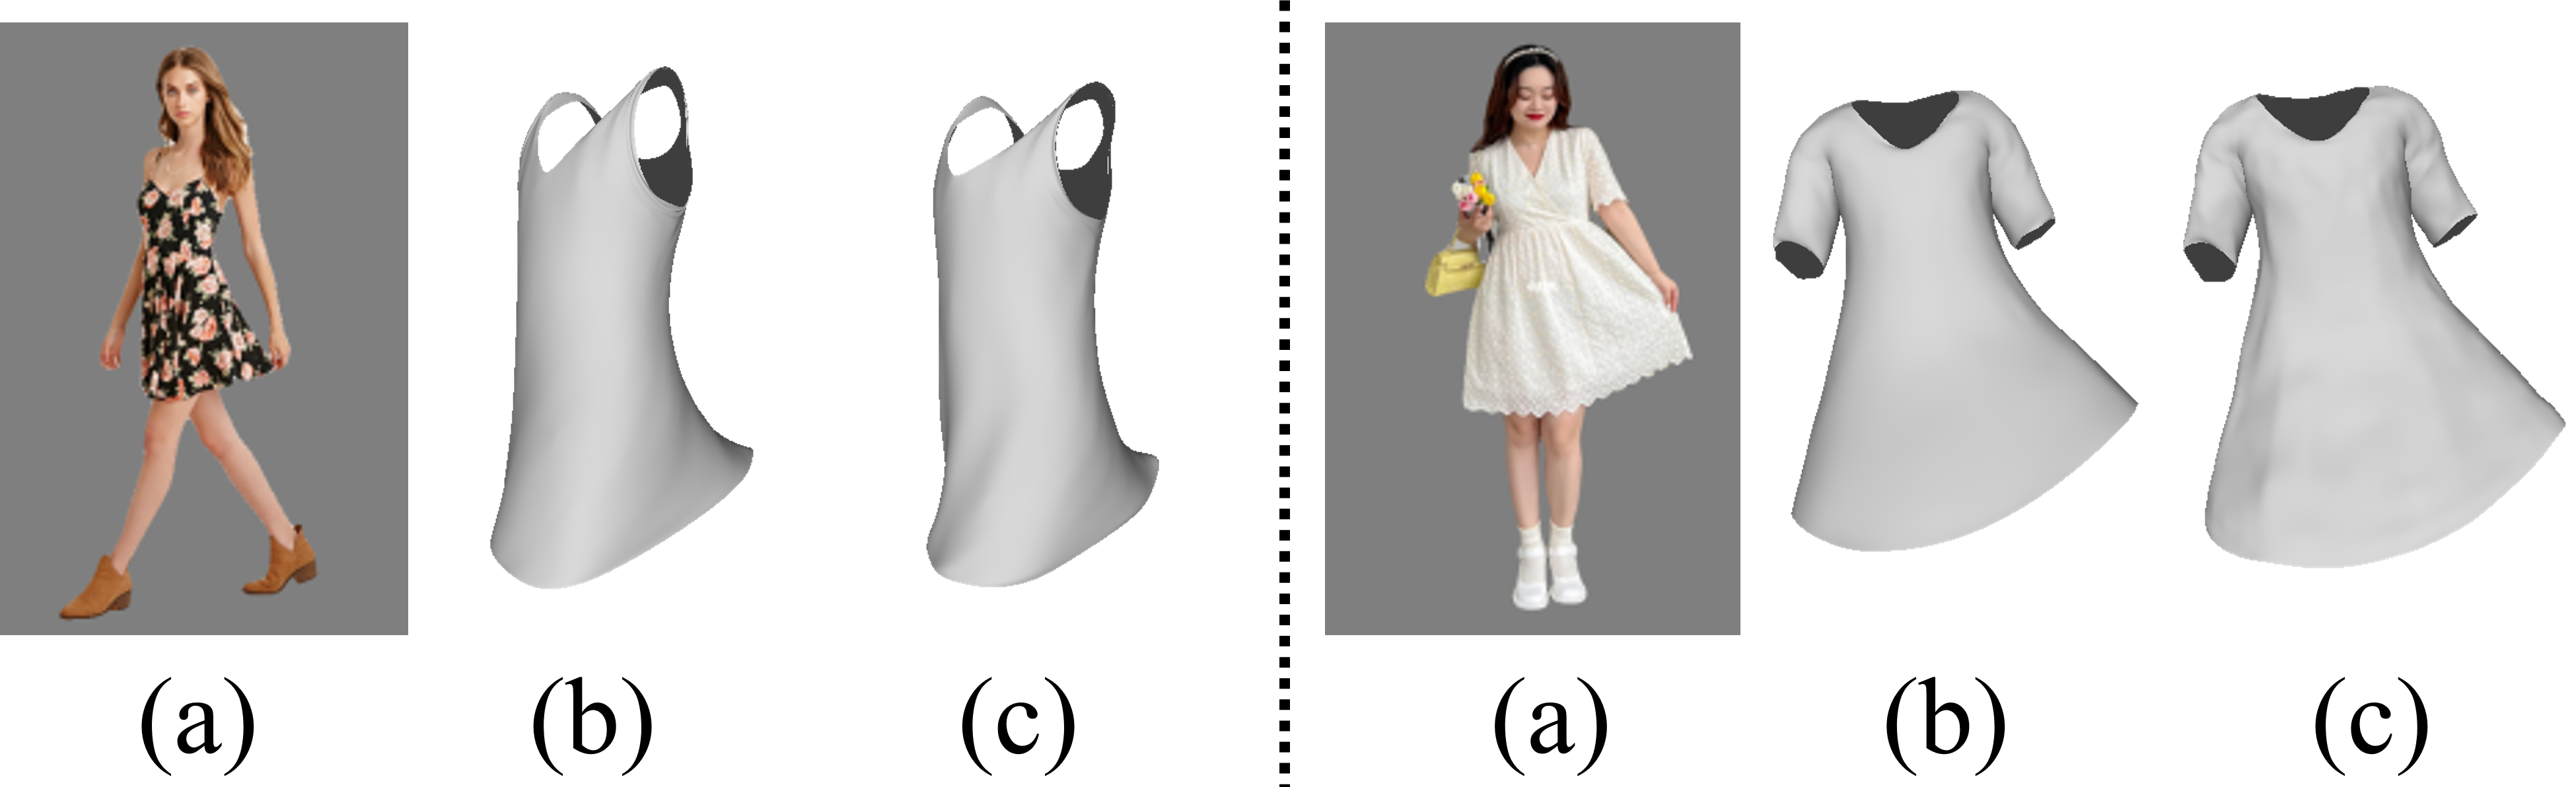}
      \caption{Qualitative comparisons of our method trained on data without geometric details (b) and with geometric details (c).}
  \label{fig:wr_training_result}
\end{figure}
