# Supplementary material for: MVImgNet2.0: A Larger-scale Dataset of Multi-view Images
Source: arXiv:2412.01430 source file (2024-12-02)
Supplement: Supplementary file 8 [file table_ablation2.tex]

\begin{table}[htbp]
    
    \centering
    \resizebox{0.49\textwidth}{!}{
        \begin{tabular}{l|c|c|c}
        % \hline 
        \toprule
        Method & Displacement & Feature Lines & Ours \\
        \midrule
        Chamfer-$L_2$ $\downarrow$ & 14.329 & 12.616 & \textbf{7.625} \\
        \midrule
        Normal-Consis. $\uparrow$  & 0.829  & 0.841 & \textbf{0.916} \\
        \bottomrule
        \end{tabular}
    }
    \caption{Quantitative comparison between our method and alternative strategies for modeling pose-independent meso-scale deformation. Our method achieves the best results in terms of Chamfer-$L_2$ and Normal Consistency.}
    \label{tab:ablation2}
    \vspace{-3mm}
\end{table}
