# Supplementary material for: MVImgNet2.0: A Larger-scale Dataset of Multi-view Images
Source: arXiv:2412.01430 source file (2024-12-02)
Supplement: Supplementary file 9 [file table_dataset.tex]

\begin{table}[htbp]
    
    \centering
    \resizebox{0.49\textwidth}{!}{
        \begin{tabular}{l|c|c|c|c|c}
        % \hline 
        \toprule
        Category & Dress & Coat & Skirt & Top & Pant \\
        \midrule
        Total & 1,571 & 1,427 & 1,049 & 1,501 & 452 \\
        \bottomrule
        \end{tabular}
    }
    \caption{Data statistics for each garment category.}
    \label{tab:dataset}
\end{table}
