# Supplementary material for: MVImgNet2.0: A Larger-scale Dataset of Multi-view Images
Source: arXiv:2412.01430 source file (2024-12-02)
Supplement: Supplementary file 10 [file supplementary.tex]

\documentclass[acmtog]{acmart}
\acmSubmissionID{905}

\usepackage{booktabs} % For formal tables
\usepackage{amsfonts}

\usepackage{makecell}
\usepackage{multirow}

% TOG prefers author-name bib system with square brackets
\citestyle{acmauthoryear}
%\setcitestyle{nosort,square} % nosort to allow for manual chronological ordering

\usepackage[ruled]{algorithm2e} % For algorithms

\SetAlFnt{\small}
\SetAlCapFnt{\small}
\SetAlCapNameFnt{\small}
\SetAlCapHSkip{0pt}

\usepackage{enumitem}

% Metadata Information
\acmJournal{TOG}
%\acmVolume{38}
%\acmNumber{4}
%\acmArticle{39}
%\acmYear{2019}
%\acmMonth{7}

% Copyright
%\setcopyright{acmcopyright}
%\setcopyright{acmlicensed}
%\setcopyright{rightsretained}
%\setcopyright{usgov}
%\setcopyright{usgovmixed}
%\setcopyright{cagov}
%\setcopyright{cagovmixed}

% DOI
%\acmDOI{0000001.0000001_2}

% Paper history
%\received{February 2007}
%\received{March 2009}
%\received[final version]{June 2009}
%\received[accepted]{July 2009}

% \newcommand{\hb}[1]{{\color{purple}            {#1}}}
% \newcommand{\hbc}[1]{{\color{cyan}            {[HB: #1]}}}

% \newcommand{\han}[1]{
% 	\textbf{\color{red}{[HAN: #1]}}
% }

% Document starts
\begin{document}
% Title portion
\title{MVImgNet2.0: A Larger-scale Dataset of Multi-view Images - Supplemental Material}

\setcopyright{acmlicensed}
\acmJournal{TOG}
\acmYear{2024} \acmVolume{43} \acmNumber{6} \acmArticle{} \acmMonth{12}\acmDOI{10.1145/3687973}
% \keywords{3D character modeling, 3D Dataset}

\maketitle

\input{supp/11_data}
\input{supp/12_exp}

\bibliographystyle{ACM-Reference-Format}
\bibliography{reference}

\end{document}
