# Supplementary material for: MVImgNet2.0: A Larger-scale Dataset of Multi-view Images
Source: arXiv:2412.01430 source file (2024-12-02)
Supplement: Supplementary file 11 [file fig_data_template.tex]

\begin{figure}[htbp]
  \centering
  \includegraphics[width=.98\linewidth]{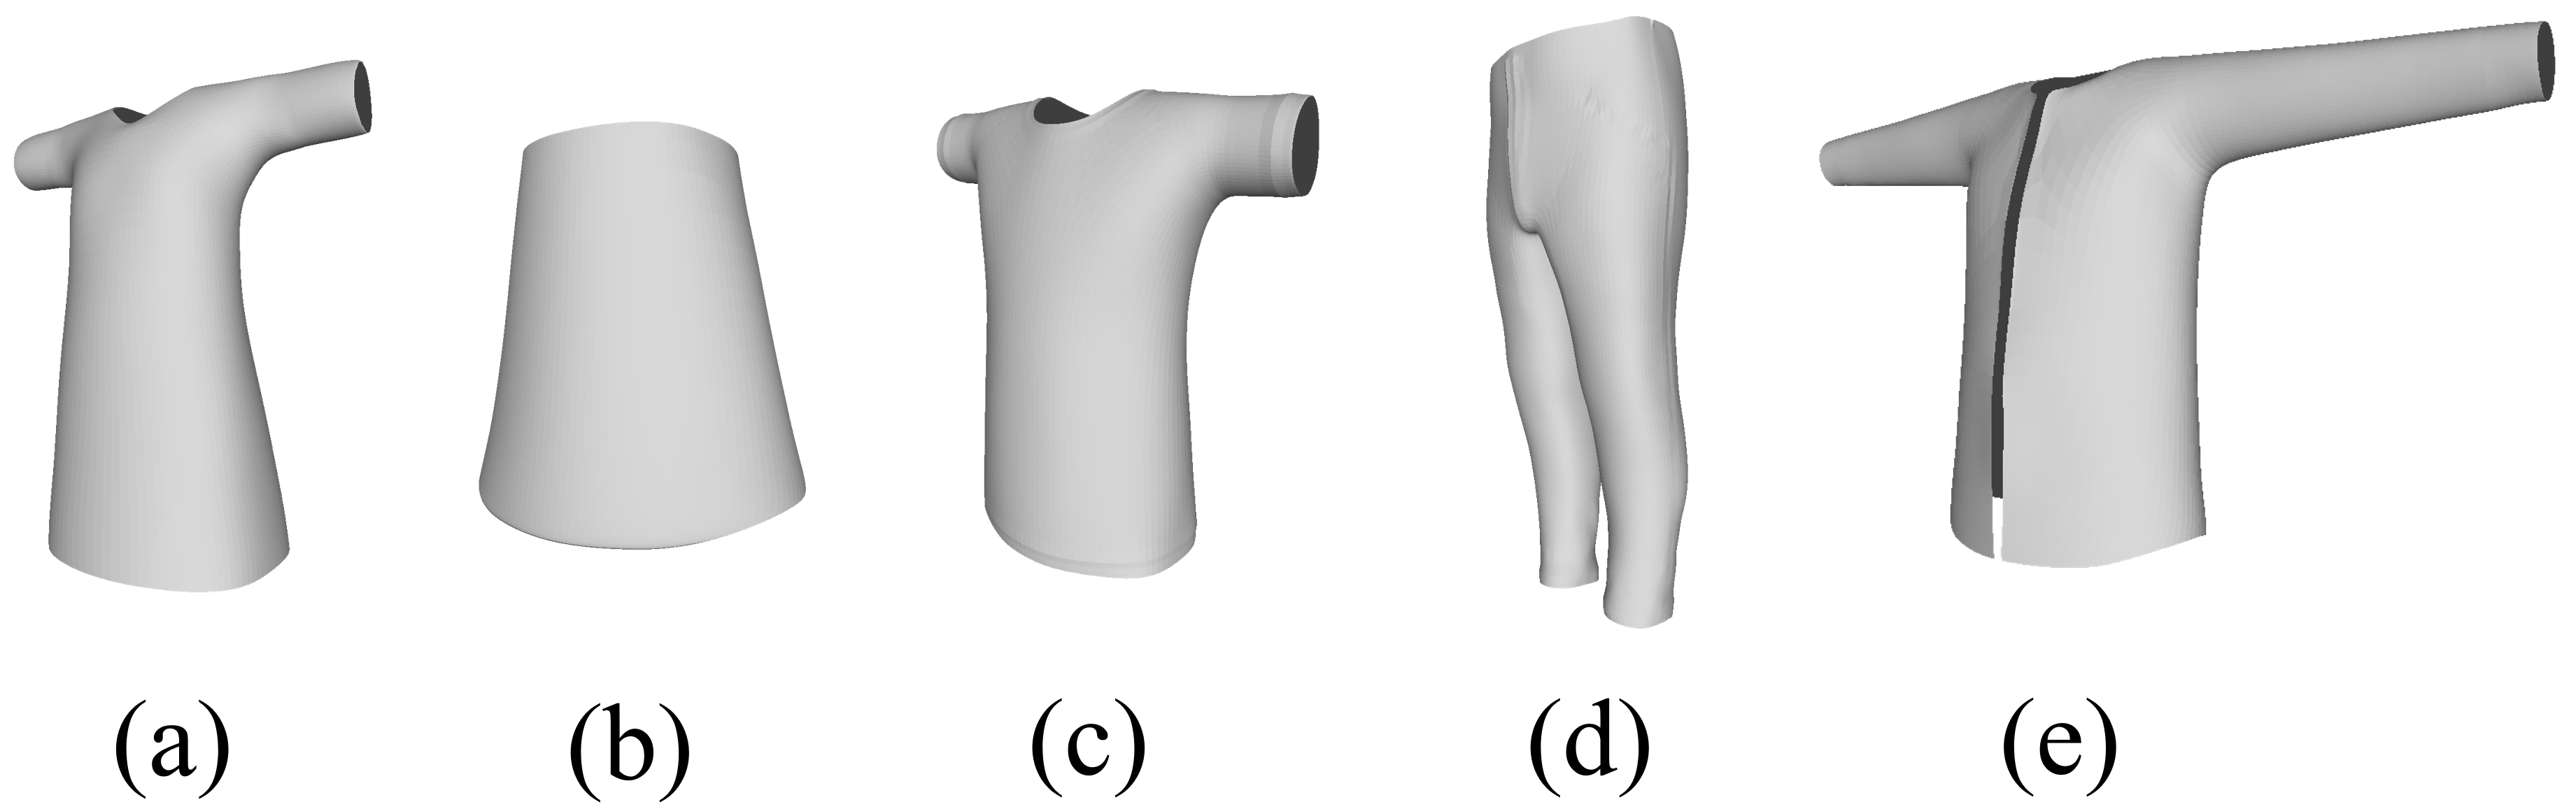}
  \caption{Predefined templates for each garment category, including (a) dress, (b) skirt, (c) top, (d) pant, and (e) coat.}
  \label{fig:data_template}
\end{figure}
